# Supplementary material for: Distributed Mapping with Privacy and Communication Constraints: Lightweight Algorithms and Object-based Models
Source: arXiv:1702.03435 source file (2017-02-11)
Supplement: Supplementary file 1 [file appendix.tex]

\appendix

\subsection{Convergence of \DJ in The Rotation Subproblem~\eqref{eq:normEq-R}}

\begin{proposition}[Convergence in Rotation Subproblem]
\label{prop:convergenceRotation}
Assume that we have $n$ robots, each one having a single pose/rotation.
Then the distributed Jacobi algorithm, applied to the rotation estimation 
subproblem~\eqref{eq:normEq-R} asymptotically converges to the centralized solution
$\vr^c = (\MA_r\tran \MA_r)\inv \MA_r\tran \vb_r$.
\end{proposition}

In this appendix we prove Proposition~\ref{prop:convergenceRotation}.
To make notation more compact, we define $\MH_r \doteq \MA_r\tran \MA_r$
and $\vg_r \doteq \MA_r\tran \vb_r$, such that the linear system we want to solve becomes:
\beq
\label{eq:app:rot}
\MH_r \vr = \vg_r
\eeq
Let us start by recalling that the \DJ iterations can be written in compact form 
as:
\beq
\label{eq:app:DJrot}
\vr\at{k+1} = \MD_r\inv \left(\MN_r \vr\at{k} + \vg_r\right)
\eeq
where $\MD_r \doteq \text{blockDiag}(\MH_r)$ (where blockDiag returns the $9\times 9$ diagonal blocks of $\MH_r$)
and $\MN_r \doteq \MD_r - \MH_r$. 
It is known that the Jacobi iterations~\eqref{eq:app:DJrot} converge 
to the solution of~\eqref{eq:app:rot} from any initial condition $ \vr\at{0}$ if and 
only if the spectral radius $\rho(\MD_r\inv \MN_r) < 1$~\cite[page 144]{Bertsekas89book}.\footnote{The 
spectral radius $\rho(\MM)$ of a matrix $\MM \in \Real{n \times n}$ is 
$\rho(\MM) \doteq \max\{|\lambda_1|,\ldots,|\lambda_n|\}$, 
where $\lambda_i$ is the $i$-th eigenvalue of $\MM$.}

We establish $\rho(\MD_r\inv \MN_r) < 1$ in 3 steps. First, we discuss
 the structure of $\MH_r$; second, leveraging the structure of $\MH_r$, we bound $\rho(\MD_r\inv \MN_r)$ with the 
 spectral radius of a matrix that is easier to analyze, i.e., $\rho(\MD_r\inv \MN_r) \leq \rho(\MU_r)$; 
 %(the \emph{matricial norm} matrix); 
 finally, we establish that $\rho(\MU_r) < 1$, from which the result follows.

 \begin{enumerate}
 \item \emph{Structure of $\MH_r$}. Recall that $\MH_r \doteq \MA_r\tran \MA_r$ 
 and that we defined $\MA_r$ such that:
\beq
\label{eq:app:rot0}
% \sum_{(\alpha_i,\beta_j) \in \calE} \omegaR \normsq{ \MR\of{\beta}{j} \!\!-\! \MR\of{\alpha}{i} \MRbar\subs}{\frob} 
\sum_{(\alpha,\beta) \in \calE} \omegaR \normsq{ \MR\of{\beta}{} \!\!-\! \MR\of{\alpha}{} \MRbar_{\beta}^{\alpha} }{\frob} 
= 
\|\MA_r \vr - \vb_r \|^2  
\eeq
where we dropped the time indices for simplicity (we are assuming that each agent has a single rotation).

\renewcommand{\vec}[1]{\text{vec}\left(#1\right)}

Let us manipulate the left-hand-side of the previous expression to make this conversion more explicit.
For this purpose, we observe that:
\beq
\label{eq:app:vectorizeNorm}
\normsq{ \MR\of{\beta}{} \!\!-\! \MR\of{\alpha}{} \MRbar_{\beta}^{\alpha} }{\frob}  =
\normsq{  \vec{ 
\MR\of{\beta}{} \!-\! \MR\of{\alpha}{} \MRbar_{\beta}^{\alpha} 
} }{}  
\eeq
where $\vec{\cdot}$ vectorize a matrix by columns. The following 
equalities follow from basic properties of the $\vec{\cdot}$: 
\beq
\label{eq:app:chain}
\begin{array}{rl}
& %\sum_{(\alpha,\beta) \in \calE} \omegaR 
\normsq{  \vec{ 
\MR\of{\beta}{} \!-\! \MR\of{\alpha}{} \MRbar_{\beta}^{\alpha} 
} }{}  
= \\
\substack{ \grayMath{(\|\MM\|_\frob = \|\MM\tran\|_\frob)} } & 
% \sum_{(\alpha,\beta) \in \calE} \omegaR 
\normsq{  \vec{ 
\MR\tran\of{\beta}{} \!-\! (\MRbar_{\beta}^{\alpha})\tran \MR^\tran\of{\alpha}{}  
} }{}  
= \\
\substack{ \grayText{(linearity)} } &
% \sum_{(\alpha,\beta) \in \calE} \omegaR 
\normsq{  
\vec{ \MR\tran\of{\beta}{} } \!-\! 
\vec{ (\MRbar_{\beta}^{\alpha})\tran \MR^\tran\of{\alpha}{}  } }{} 
= \\
\substack{ \grayMath{ (\MA,\MB \in \Real{d \times d}, \; \vec{\MA \MB} =} \\ = \grayMath{ (\eye_d \kron \MA) \vec{\MB}) } }  &
% \sum_{(\alpha,\beta) \in \calE} \omegaR 
\normsq{  \vec{ 
\MR\tran\of{\beta}{} } \!-\! 
\MQbar_{\beta}^{\alpha} \; 
\vec{ \MR\tran\of{\alpha}{} } }{} 
\end{array}
\nonumber
\eeq
with $\MQbar_{\beta}^{\alpha} \doteq \eye_3 \kron \MRbar_{\beta}^{\alpha}$.
Chaining the equalities~\eqref{eq:app:chain} and~\eqref{eq:app:vectorizeNorm}, 
and defining $\vr_\alpha \doteq \vec{\MR\tran_\alpha}$ ($\vr_\alpha$ is a vector 
stacking the entries of $\MR\tran_\alpha$ by rows), 
we rewrite~\eqref{eq:app:rot0} as:
\beq
\sum_{(\alpha,\beta) \in \calE} \omegaR \normsq{ \MR\of{\beta}{} \!\!-\! \MR\of{\alpha}{} \MRbar_{\beta}^{\alpha} }{\frob} 
= 
\sum_{(\alpha,\beta) \in \calE} \omegaR  \normsq{  \vr\of{\beta}{} - \MQbar_{\beta}^{\alpha} \; \vr\of{\alpha}{} }{} 
\eeq

 [Kierzkowski11ejla-geshgorinDisks]

 \end{enumerate}
